# Supplementary material for: Automated Code Editing with Search-Generate-Modify
Source: arXiv:2306.06490 source file (2024-02-26)
Supplement: Supplementary file 1 [file appendix.tex]

\section{Appendix}

\subsection{Examples of correct and incorrect modification/generation}
\begin{figure}[h!]
     \centering
     \begin{subfigure}[b]{0.5\textwidth}
         \centering
         \includegraphics[width=\textwidth]{figures/Appendix_success_edit.pdf}
         \caption{Csv-12}
         \label{fig:appendix_succefful_modification}
     \end{subfigure}
     \hfill
     \begin{subfigure}[b]{0.5\textwidth}
         \centering
         \includegraphics[width=\textwidth]{figures/Appendix_unsuccessful_edit.pdf}
         \caption{JacksonDatabind-57}
         \label{fig:appendix_unsuccessful_modification}
     \end{subfigure}
     \hfill
        \caption{Examples of successful modification (Csv-12) and unsuccessful modification (JacksonDatabind-57) }
        \label{fig:rq1-case-study}
\end{figure}

\begin{figure}
     \centering
     \begin{subfigure}[b]{0.5\textwidth}
         \centering
         \includegraphics[width=\textwidth]{figures/Appendix_successful_generate.pdf}
         \caption{Jsoup-51}
         \label{fig:appendix1}
     \end{subfigure}
     \hfill
     \begin{subfigure}[b]{0.5\textwidth}
         \centering
         \includegraphics[width=\textwidth]{figures/Appendix_unsuccessful_generate.pdf}
         \caption{JacksonDatabind-27}
         \label{fig:appendix_unsuccessful_generation}
     \end{subfigure}
     \hfill
        \caption{Examples of successful modification (Jsoup-51) and unsuccessful generation (JacksonDatabind-27) }
        \label{fig:appendix2}
\end{figure}
